# Supplementary material for: Fault Tolerance by Construction
Source: arXiv:2506.17181 source file (2026-03-31)
Supplement: Supplementary file 1 [file 01-error-detector-model.tex]

\section{Error detector model under fault-aware rewrites}
\label{appendix:error-detector-model}
Given a ZX diagram with ZX distance $d$, we can detect errors of weight up less than $d$ and, by \autoref{thm:correcting-circuits}, correct errors of weight up to $\lfloor \frac{d - 1}{2} \rfloor$. 
In this appendix, we will give a slightly more extensive introduction to how this might look like in practice. 
For this, we will primarily build on the error-detector model~\parencite{gidneyStimFast2021, higgottSparseBlossom2025} pedagogically introduced by \textcite{derksDesigningFaulttolerant2024}.
We will first give outline the procedure to generate the error-detector model for a given (Clifford) ZX diagram and then explore how the error-detector model changes under rewrites. 

The error-detector model consists of a representation of the decoding problem for circuits. 
We define: 
\begin{definition}[Error-detector model]
  Given a ZX diagram $D$, the error-detector model of that ZX diagram is a bipartite graph consisting of all possible edge flips on $D$ and all detection regions of $D$. 
  An edge flip is connected to a detecting region, if and only if it violates the detecting region. 
\end{definition}

Given the information which detecting regions an edge flip violates, we can calculate the syndrome of any fault, i.e.\@ set of edge flips, by calculating the parity of the violations for each detecting regions of the edge flips that the fault consists of.
A fault is detectable if at least one detecting region is violated. 

The decoding problem then consists of, given the information which detecting regions are violated, identify the most likely equivalence class of errors that could have lead to this syndrome. 
If the distance of the original ZX diagram is $d$, then we are guaranteed that all faults of weight at most $\lfloor \frac{d - 1}{2} \rfloor$ have a unique syndrome. 

Usually, the error-detector model quantum circuit can be calculated using the stabiliser formalism~\parencite{gottesmanHeisenbergRepresentation1998}.
For time-neutral ZX diagrams, we can instead use the equally polynomial-time efficient method provided by \textcite{borghansZXcalculusQuantumStabilizer2019}. 
While the provided method is primarily framed to calculate the stabilisers of a ZX diagram, by further restricting the output nodes to not fire, we efficiently calculate all detecting regions. 
In the error-detector model, we then chose a generating set of the detecting regions --- while this choice does not impact the distance of the corresponding circuit, it might affect the efficiency of the decoder. 

\textcolor{green}{slightly more explanation?}
Fault-aware rewrites are guaranteed to preserve the ZX distance of a diagram.
Therefore, if we have some diagram $D$ with distance $d$ and use a fault-$d$-preserving rewrite to obtain a new diagram $D'$, we can use the method above to calculate a new error-detector model for $D'$. 
More generally, however, one could explore how fault-aware rewrites impact the error-detector model of a given graph and whether they preserve desirable properties. 
We will leave  this as future work.
