# Supplementary material for: Fault Tolerance by Construction
Source: arXiv:2506.17181 source file (2026-03-31)
Supplement: Supplementary file 2 [file 02-outcomes-from-ft-syndrome-extraction.tex]

\section{How to interpret measurement outcomes after FT rewrites}
In \autoref{sec:fault-tolerant-syndrome-extraction} we provide methods of fault-tolerantly doing syndrome extraction. 
Depending on ones choice, the resulting cirucit uses four or two measurements to implement a single weight-four measurement. 
One obvious question is how to derive the measurement outcome of the weight-four measurement from this implementation. 

There are two different answers to this. 
Answer one boils down to: maybe you shouldn't. 
Given that we have derived these implementations using fault-aware rewrites, we know that the distance of the original circuit is being preserved. 
Therefore, we know that if we replace the idealized measurement in the circuit by these implementations, the distance will be preserved.
Thus, we can simply calculate a new error-detector model as outlined in \autoref{appendix:error-detector-model} and solve the resulting, new decoding problem. 

However, as observed above, the new error-detector model might have different properties that make it more difficult to decode and we want to instead use our original decoder. 
In that case, we have to revert to the second answer: can can calculate the outcome of the original measurement based on the new implementation. 
For this, we assume that we live in a fault-free setting, meaning we can use the usual ZX calculus. 
The question remains, given the two outcomes of our newly derived circuit, how do we calculate the outcome of the syndrome measurement. 
For this, we have to parameterise all measurement. 
We get: 
\[\tikzfig{TODO}\]
We can now undo the rewrites we originally did to get this measurement: 
\[\tikzfig{TODO}\]

Thus, we see that the outcome of the original measurement is the parity of the two measurements. 
Furthermore, we see that we only implement the measurement up to Paulis which are determined by the measurement outcomes. 
Therefore, we have to keep track of this and update our Pauli frames accordingly. 
In Clifford circuits, this is efficiently doable and in a non-Clifford setting we have to take more care to correct errors either way. 

However, some rewrites introduce new detecting regions. 
For example, in \textcite{rodatzFloquetifyingStabiliser2024}, we propose to implement the cat-like linear map using two consecutive Pauli measurements as follows: 
\[\tikzfig{TODO}\]

If we apply the same routine, we get: 
\[\tikzfig{TODO}\]

Here, we get a free floating spider with scalar $(r_1 + r_2) \pi$. 
If $r_1 \not= r_2$, then this is equal to a free-floating spider with a scalar of $\pi$, meaning we have a global phase of 0. 
This means that our newly created detecting region has detected an error. 
At this point, all bets are off --- we have to refer back to the first answer. 
If this detecting region is violated, the original decoder can not be used here anymore.
