# Supplementary material for: Fault Tolerance by Construction
Source: arXiv:2506.17181 source file (2026-03-31)
Supplement: Supplementary file 3 [file 03-knill-error-correction.tex]

\section{Knill-style error correction}
\label{appendix:knill}
Shor-style syndrome extraction and Steane-style syndrome extraction treat the decoding problem as separate steps, first doing the syndrome extraction and then doing the decoding and correction. 
Knill-style error correction does not separate these steps, instead performing them as one. 
In other words, Shor- and Steane-style syndrome extraction could be performed without the correction, leaving the logical data in the same state as before. 
Knill-style error correction can not do this. 
If one skips the decoding and correction associated with Knill-style error correction one will have brought the data back to the code space, however, potentially introduced a logical error. 
Thus, the goal of the decoding is not to identify the physical error introduced by the noise but rather the logical error introduced by the teleportation. 
This means that the corrections one applies in Knill-style syndrome extraction do not correspond to physical errors, i.e.\@ Paulis of weight less than $d$ but rather logical operations, i.e.\@ Paulis of weight at least $d$.

We can show the correctness of Knill-style error correction using fault-aware rewrites. 
In this case, showing correctness involves showing that it is fault-equivalent to the FTEC box, i.e.\@ fault-equivalent to:
\[\tikzfig{appendix/knill/ftec-box}\]

Knill-style error correction consists of preparing the Bell state over two logical code blocks, transversally entangling it with the data and then performing transversal, destructive measurements on the first two code blocks. 
We have: 
\[\tikzfig{appendix/knill/knill-error-correction}\]
The first step of this derivation follows from~\parencite[Chapter 12.4.1]{gottesmanSurvivingQuantum2024}.
At this point in time, we have not yet attempted to recover it in terms of fault-aware rewrites. 
The next step follows from the assumption that the corrections are implemented fault-tolerantly. 
Then we can remove the encoders followed by the decoders by the properties of quantum error correction codes. 
Using spider fusion and only connectivity matters, we can rearrange the circuit to act on one code block. 
Finally, we observe that the logical Paulis cancel each other out. 
Thus, we have shown that Knill-style syndrome extraction is in fact fault-equivalent to the specification of an FTEC box and therefore correct.
