# Supplementary material for: Fault Tolerance by Construction
Source: arXiv:2506.17181 source file (2026-03-31)
Supplement: Supplementary file 4 [file 04-gottesman-ft.tex]

\section{Gadget-Based Fault Tolerance using Fault Equivalence}
\textcolor{red}{TODO: fix up}

Gadget-based fault-tolerant protocols construct fault-tolerant implementations of ideal logical circuits by replacing logical operations by fault-tolerant gadgets.
For the remainder of this section, we formalize a gadget-based protocol in terms of $d$-fault equivalence with slightly more permissive criteria than those of \textcite{gottesmanSurvivingQuantum2024}.

Closely mirroring the definition of \textcite{gottesmanSurvivingQuantum2024}, we can use an error-correcting code to define a gadget-based fault tolerance protocol as:
\begin{definition}[Gadget-based fault-tolerant protocol]
    A \emph{gadget-based fault-tolerant protocol} is defined relative to a distance $d$ QEC code ($enc, dec$) along with the following fault-tolerant gadgets:
    \begin{itemize}
        \item Gate gadgets
        \begin{itemize}
            \item State preparation gadget for at least one type of state
            \item Measurement gadget for at least one type of measurement
            \item Gate gadget for a universal gate set
        \end{itemize}
        \item Error correction gadget
    \end{itemize}
\end{definition}

The goal is to replace all the gates by their fault-tolerant gadgets interlaced with error correction gadgets to get the encoded, fault-tolerant circuit.
Thus, each of these gadgets has to satisfy certain behavioural requirements in a faulty setting.

%Gadget-based fault-tolerant protocols are defined with respect to a quantum error correction code $enc$, for which we know that there exists a decoder such that:
%\[\tikzfig{04-fault-tolerance/def-qec-dist-preserv}\]

We can view a quantum error correction code as encoding the trivial computation, i.e.\@ idling.
However, in an actual computation, we want to be able to perform operations.
But performing computations on encoded data might spread errors unfavourably or introduce new ones.
Therefore, gadgets that perform a computation on encoded data have to satisfy certain constraints.
For example, consider some operation $g_1$ on one code block of $k$ logical qubits.
We say, $\overline{g_1}$ is a fault-tolerant gadget for $g_1$, if it satisfies the following $d$-fault equivalence:
\[\tikzfig{04-fault-tolerance/def-ft-gadget-single-qubit}\]

Applying the $d$-fault equivalence definition:
any fault within the composed diagram must either be detectable or correspond to a fault within the ideal logical gate diagram.
As an ideal gate permits only the trivial fault, any undetectable fault $\mathcal{F}$ in the implementation with $wt(\mathcal{F}) < d$ must result in the correct logical operation.
This ensures low-weight faults do not cause logical errors.

More generally, we can define:
\begin{definition}[$d$-Fault-Tolerant Gadget Implementation]
    \label{def:fault-tolerance}
    Given a quantum error correction code $enc: \mathbb{C}^{2^k} \to \mathbb{C}^{2^n}$ with its ideal decoder $dec: \mathbb{C}^{2^n} \to \mathbb{C}^{2^k}$ and a logical operation $g: (\mathbb{C}^{2^k})^{m_i} \to (\mathbb{C}^{2^k})^{m_o}$ from $m_i \in \mathbb{N}$ input code blocks to $m_o \in \mathbb{N}$ output code blocks, a $d$-fault-tolerant implementation of $g$ is a quantum circuit $C_{\overline{g}}: (\mathbb{C}^{2^n})^{m_i} \to (\mathbb{C}^{2^n})^{m_o}$ such that there exists a ZX diagram $\overline{g}$ that is fault-accounting for $C_{\overline{g}}$ and satisfies the following $d$-fault equivalence condition:
    \[\tikzfig{04-fault-tolerance/def-ft-gadget}\]
\end{definition}
\noindent
For $m_i = m_o = 1$ and $g = id$, we are left with a single encoder followed by the ideal decoder which trivially holds by the properties of the quantum error correction code.

More generally, though, our definition of a fault-tolerant gadget captures substantially more cases.
In particular, having given it for an arbitrary number of input and output code blocks, this definition encapsulates many special cases we might be interested in.
For example, for a universal gate set consisting of operations of weight one and two, we need to find fault-tolerant gadgets satisfying the conditions depicted below:
\begin{align*}
    \text{\small State: } \quad \resizebox{0.28\columnwidth}{!}{\tikzfig{04-fault-tolerance/def-ft-gadget-state-prep}} && \text{\small Single-qubit gate: } \quad \resizebox{0.35\columnwidth}{!}{\tikzfig{04-fault-tolerance/def-ft-gadget-single-qubit}}\\
    \text{\small Measurement: } \quad \resizebox{0.28\columnwidth}{!}{\tikzfig{04-fault-tolerance/def-ft-gadget-measurement}} && \text{\small Two-qubit gate: } \quad \resizebox{0.35\columnwidth}{!}{\tikzfig{04-fault-tolerance/def-ft-gadget-two-qubit}}\\
\end{align*}

Assuming that we have found such fault-tolerant implementations for all the operations we want to perform, we can replace the individual gates in our original, idealized circuit.
For the sake of simplicity, we assume that the code of our choice encodes one logical qubit per code block, i.e.\@ $k = 1$.
This replacement yields a diagram $d$-fault-equivalent to the original ideal circuit diagram:
\begin{center}
    \resizebox{\columnwidth}{!}{
         \tikzfig{04-fault-tolerance/ft-ideal-circuit} $\underset{\tiny fault-d}{=}$ \tikzfig{04-fault-tolerance/dist-rewrite-ideal-circuit}}
\end{center}
\noindent
This rewritten structure, composed of FT gate gadgets, forms the core of the implementation.
However, standard protocols interleave these with explicit fault-tolerant error correction steps.

The final necessary component is the fault-tolerant error correction gadget:
\begin{definition}[Fault-tolerant error correction]
    \label{def:ftec}
    Given a quantum error correction code $enc: \mathbb{C}^{2^k} \to \mathbb{C}^{2^n}$ with distance $d$, a fault-tolerant error correction gadget is a quantum circuit $C_{FTEC}: \mathbb{C}^{2^n} \to \mathbb{C}^{2^n}$ such that there exists a ZX diagram $FTEC$ that is fault-accounting for $C_{FTEC}$ and satisfies the following condition:
    \[\tikzfig{04-fault-tolerance/def-ftec}\]
\end{definition}
\noindent
Using this final gadget, we get the full structure:
\[\tikzfig{04-fault-tolerance/rewriting-circuit-final}\]

Thus, if we have quantum circuits that fault-tolerantly implement each of these gadgets, we have our encoded fault-tolerant circuit.
In particular, we are guaranteed that any combination of faults in the circuit corresponds to at most as many edge flips in the corresponding ZX diagram.
As this ZX diagram is defined to be $d$-fault-equivalent to the idealized fault-free diagram, any combination of less than $d$ faults must be detectable, achieving a $d$-fault-tolerant implementation of the circuit.

Readers familiar with Gottesman's gadget-based fault-tolerance protocol might recognise the extended rectangles~\parencite{gottesmanSurvivingQuantum2024}.
However, to fully show the relationship of our protocol to Gottesman's, we have to relate the respective fault-tolerance conditions for the gadgets which we will do, amongst other things, in the following section.

\section{Gottesman}
\label{appendix:gottesmans-ft}
In this section, we will relate the sufficient condition of fault-tolerance given in \autoref{def:ft-conditions} to the conditions given by \textcite{gottesmanSurvivingQuantum2024}.
For this, we will first restate the conditions and alternatively express them in terms of effects on errors by expanding the definition of $d$-fault equivalence. 
Using this, we can formally show equivalence to Gottesman's conditions. 
We observe that for two-qubit gates we can express an equivalent condition in terms of the expanded notation, however, at the moment not in terms of basic fault equivalences, suggesting that there are additional desirable properties fault equivalences currently do not capture.  

\subsection{Full characterisation}
In \autoref{sec:errors-to-FT} we gave a characterisation of fault-tolerance in terms of \emph{correctness}, \emph{push-through} and \emph{push-out} for physical gadget acting on one code block. 
We defined fault-tolerance as: 
\begin{definition}
    \label{def:fault-tolerance}
    Given a quantum error correction code $enc: \mathbb{C}^{2^k} \to \mathbb{C}^{2^n}$ with distance $d$ and a logical operation $g: (\mathbb{C}^{2^k})^{m_1} \to (\mathbb{C}^{2^k})^{m_2}$, a fault-tolerant implementation of $g$ is an operation $\overline{g}: (\mathbb{C}^{2^n})^{m_1} \to (\mathbb{C}^{2^n})^{m_2}$ such that: 
    \[\tikzfig{05-fault-tolerance/def-ft-gadget}\]
\end{definition}

- sufficient condition

- show that it is sufficient

An alternative characterisation of the three sufficient conditions is the following: 
\begin{align*}
    \eqref{correctness}: \tikzfig{correctness} \\
    \eqref{push-out}: \text{for all } \mathcal{F} \text{ with } |\mathcal{F}| < d \\
\end{align*}

\subsection{Gottesman's definition}
To give Gottesman's definition of fault-tolerance, we first have to define: 
\begin{definition}{r-filter~\parencite[Def. 10.7, p. 166]{gottesmanSurvivingQuantum2024}}
 The \textit{r-filter} for the QECC $Q$ is the projector on the subspace spanned by states of the form $E\ket{\psi}$, where $\ket{\psi} \in Q$ and $E$ is an error of weight at most $r$. We have: 
    \[\tikzfig{fault-tolerance/r-filter}\]
\end{definition}

\subsection{Equivalence of the definitions}
