# Supplementary material for: Fault Tolerance by Construction
Source: arXiv:2506.17181 source file (2026-03-31)
Supplement: Supplementary file 5 [file 06-measurement-outcomes-V1.tex]

\section{Measurement Outcomes in ZX Diagrams}
In the main body, we treat ZX diagrams as linear maps.
In practice, ZX diagrams implement non-deterministic computations.
In this appendix, we formalise the role of measurements in ZX diagrams.
Using this framework, we redefine three notions that are essential for our paper: detectability of faults, equivalence of diagrams, and fault equivalence of diagrams.
We then show that the definitions used in the main body are satisfied if and only if their counterparts for non-deterministic computations are satisfied.
This result justifies the simplified treatment of ZX diagrams as linear maps adopted in the main body.
The key takeaway is that measurements need not be tracked explicitly during derivations.

Furthermore, we provide the necessary tools to replace one Clifford subcircuit with another and give ways of interpreting the corresponding measurement outcomes.
Importantly, in the noise-free case, we never need any post-selection for one equivalent ZX diagram to take the place of another.

Before proceeding, we introduce some additional terminology.
In \autoref{sec:detection-regions}, we introduced Pauli webs and highlighted the special role of detecting regions, that is, Pauli webs that act trivially on the boundary edges.
For the treatment of measurement outcomes, however, it is necessary to consider all Pauli webs.
We therefore introduce the following terminology:
\begin{definition}[Stabilising, co-stabilising, and logical Pauli webs]
    Let $D$ be a ZX diagram.  
    A Pauli web $P \in \overline{\mathcal{P}^{|E|}}$ is called
    \begin{itemize}
        \item a \emph{stabilising Pauli web} if it acts trivially on all input edges,
        \item a \emph{co-stabilising Pauli web} if it acts trivially on all output edges,
        \item a \emph{logical Pauli web} if it acts nontrivially on both inputs and outputs.
    \end{itemize}
\end{definition}
\textcite{rodatzFloquetifyingStabiliser2024} show the relationship between Pauli webs and stabilisers, co-stabilisers and logicals. 
In particular, for every stabiliser of some diagram $D$, there exists a corresponding Pauli web that has the same action on the output wires. 
Similarly, the action of every stabilising Pauli web corresponds to stabilisers of $D$.

\subsection{Running ZX Diagrams}
In the main body, we treat ZX diagrams as static, linear maps. 
However, in practice, they represent quantum computations that are run on quantum computers. 
For a given input, running a computation results in classical measurement outcomes, sampled from some probability distribution, and results in a new state.

Usually, in the ZX calculus, measurement outcomes are represented as parameters on spiders. 
Instead, we will represent measurement outcomes as edge flips, that is, as special elements in $\overline{\mathcal{P}^{E}}$.
This allows us to leverage a range of insights about faults on diagrams, including work by \textcite{ruschCompletenessFault2025}.
We define: 
\begin{definition}[Measurement outcomes]
    Let $D$ be a ZX diagram.  
    A set of measurements $\mathcal{M}$ on $D$ is a set of tuples $(e, t)$ consisting of an edge $e \in E$ and a type $t \in \{X, Y, Z\}$. 
    The $0$ outcome of the measurement is represented by the trivial Pauli $I^{|E|}$.
    The $1$ outcome of the measurement is represented by the Pauli $P_{(e, t)} \in \overline{\mathcal{P}^{E}}$ that acts as $t$ on edge $e$ and trivially everywhere else. 
    Given a set of measurements $\mathcal{M}$ the set of measurement outcomes $\overline{\mathcal{P}_\mathcal{M}} = \langle P_{(e, t)}\rangle$ is defined as the group generated by all $P_{(e, t)}$ for $(e, t) \in \mathcal{M}$.
\end{definition}

For example, consider a single destructive measurement. 
As a ZX diagram, this is represented as a spider with a single input.  
To represent this measurement, we pick $\mathcal{M} = \{((1, 2), X)\}$ with $(1, 2)$ being the one edge in the diagram: 
\[
\tikzfig{appendix/measurement-outcomes}
\]
The $0$ outcome corresponds to no flip on the edge, while the $+1$ outcome corresponds to an $X$ flip before the spider. 

Throughout the rest of this appendix, unless specified otherwise, we will use $D$ to indicate non-determinisitic computations as specified by a ZX diagram $D$ while we will use $D^P$ for some $P \in \overline{\mathcal{P}^{E}}$ will be used to indicate the linear map the ZX diagram $D^P$ represents, i.e. the post-selected computation of $D$ conditioned on the measurement outcome $P$. 

We have left a lot of freedom in choosing the set of measurements on a diagram. 
This is, of course, unrealistic; we cannot deterministically implement a computation that corresponds to a projection. 
Therefore, we now have to define what we mean by a set of measurements being sufficiently expressive: 
\begin{definition}
    Let $D$ be a ZX diagram and $\mathcal M$ be a set of measurements on $D$. 
    Then we say $\mathcal M$ is complete if: 
    \[\tikzfig{appendix/measurement-completeness}\]
\end{definition}

We can now formalise the idea of running ZX diagrams:
\begin{definition}[Running a ZX diagram]
    Given a ZX diagram $D$ with a complete measurement set $\mathcal M$ and a normalised input state $\psi$, running $D$ on $\psi$ results in two pieces of information: 
    \begin{enumerate}
      \item a measurement outcome $M \in \overline{\mathcal{P}_\mathcal{M}}$ sampled from a probability distribution $\mathbb{P}_{D, \psi}$
      \item a new state $D^M \ket{\psi}$ which is conditions on the measurement outcome
    \end{enumerate}
    where $\mathbb{P}_{D, \psi}(M)$ for $M \in \overline{\mathcal{P}_\mathcal{M}}$ is given by the Born rule as: 
    \[\tikzfig{appendix/born-rule}\]
\end{definition}

Next, we define: 
\begin{definition}
    Let $\mathcal M$ be the measurement set for some diagram $D$. 
    We say a measurement outcome $M \in \overline{\mathcal{P}_\mathcal{M}}$ is valid, if there exists an input state $\psi$, such that $\mathbb{P}_{D, \psi}(M) \not= 0$. 
    We call the set of all valid measurement outcomes $valid_D \subseteq \overline{\mathcal{P}_\mathcal{M}}$. 
\end{definition}

For example, if we have two consecutive $ZZ$ measurements, in theory, there are four possible measurement outcomes: $00, 01, 10, 11$. 
However, in the noise-free case, the only two valid outcomes are $00$ or $11$, as we expect two consecutive iterations of the same projective measurement to give the same outcome. 
There exist input states for which only one of these outcomes is valid.
However, valid measurement outcomes are defined over all possible input states, meaning under the assumption that we do not know anything about the input states. 
Thus, the set of valid measurements of $D \ket{\psi}$, i.e., $D$ applied to some fixed input state, is a subset of the valid measurements of $D$.

We can characterise the set of valid measurement outcomes further. 
To study the effect of an edge flip $M$ on a diagram $D$, we can first observe that $D^I$ and $D^M$ must have the same stabilising Pauli webs \parencite{ruschCompletenessFault2025}.
The only difference between the two linear maps can therefore be whether they live in the $+1$ or $-1$ eigenspace of the corresponding stabilisers. 
Or, in other words, the effect of edge-flips is fully described by the Pauli webs they flip.

As measurements are special kinds of edge-flips, we can have a closer look at the potential effects of measurements: 
\begin{proposition}
    \label{prop:valid-outcomes}
    A measurement outcome is valid if and only if it commutes with all detecting regions.
\end{proposition}
\begin{proof}
    Let $M$ be a measurement outcome that anticommutes with a detecting region.  
    Then, by \autoref{thm:detecting-region}, we have $D^M = 0$.  
    This implies that the probability of observing $M$ is zero for every input state.  
    Hence, $M$ cannot be valid.

    Let $M$ be a measurement outcome that commutes with all detecting regions. 
    Then take any normalised state $\psi$ that lives in the $+1$ eigenspace of all the costabilisers of $D^M$. 
    Now, $\bra{\psi} D^M (D^M)^\dagger \ket{\psi}$ has no violated detecting region. 
    Therefore, it must be non-zero \parencite{ruschCompletenessFault2025} and thus, $M$ is valid. 
\end{proof}

\subsection{Finding complete measurement sets}
One key requirement for running ZX diagrams is finding a measurement set that is complete. 
Within this work, we are only interested in running quantum circuits or ZX diagrams that correspond to quantum circuits.
We prove that for any quantum circuit, the corresponding ZX diagram has an obvious, complete measurement set, namely the one that places a measurement before all the measurement operations in the quantum circuit. 

First, we prove: 
\begin{proposition}
\label{prop:measurement-completeness}
    Let $D$ be a ZX diagram, $\mathcal M$ be a measurement set, and $\mathcal{S}_c = S_1, \dots S_k$ be a generating set for all costabilising Pauli webs on $D$. 
    There exists a scalar $c$ such that $\mathcal M$ is complete for $cD$ if and only if for each $S_i$, there exists a $M_{S_i} \in valid_D$ such that such that $[M_{S_i}, S_j] = \delta_{ij}$
\end{proposition}
\begin{proof}
    First, we show that if $\mathcal M$ is complete for $cD$, then for each $S_i$ there exists a $M_{S_i} \in valid_D$ such that such that $[M_{S_i}, S_j] = \delta_{ij}$. 
    For some $S_i \in \mathcal{S}_c$, let $\psi$ be a normalised state that lives in the $-1$ eigenspace of $S_i$ and in the $+1$-eigenspace of all other $S_j$, then
    \begin{align*}
        1 = \bra{\psi}\ket{\psi} = \sum_{M \in \overline{\mathcal{P}_\mathcal{M}}} \bra{\psi} D^M (D^M)^\dagger \ket{\psi}
    \end{align*}
    But for the last expression to be non-zero, there must exist at least one $M_i$ such that $\bra{\psi} D^{M_i} (D^{M_i})^\dagger \ket{\psi}$ is non-zero. 
    But for this to be non-zero, $M_i$ must exactly satisfy $[M_{i}, S_j] = \delta_{ij}$, as otherwise, there would be a violated detecting region.
    Therefore, we have shown that for every $S_i$, there must exists a $M_{S_i} \in valid_D$ such that such that $[M_{S_i}, S_j] = \delta_{ij}$.

    Next, we will show the other direction, that if for each $S_i$, there exists a $M_{S_i} \in valid_D$ such that such that $[M_{S_i}, S_j] = \delta_{ij}$, then there must exist a scalar $c$ such that $\mathcal M$ is complete for $cD$.
    We have:
    \begin{align*}
        \sum_{M \in \overline{\mathcal{P}_\mathcal{M}}} D^M (D^M)^\dagger 
        & = \sum_{M \in valid_D} D^M (D^M)^\dagger 
        = \sum_{M \in valid_D} P_MD^IP_M^o (P_MD^IP_M^o)^\dagger \\
        & = \sum_{M \in valid_D} P_MD^IP_M^o P_M^o(D^I)^\dagger P_M 
        = \sum_{M \in valid_D}P_M D^I (D^I)^\dagger P_M
    \end{align*}
    The first step follows from the fact that non-valid measurement outcomes make $D^M$ go to zero. 
    The second step follows from \textcite{ruschCompletenessFault2025}, observing that valid measurement outcomes, as they do not violate any detecting regions, must act equivalently to some Pauli action $P_M$ on the inputs and $P_M^o$ on the outputs. 
    Given that we compose $D^M$ with its dagger, $P_M^o$ cancels out, leaving us with a Pauli action on the inputs $P_M$ that has the same effect as the measurement outcome $M$.
    
    Next, we observe that $D^I (D^I)^\dagger$ is equivalent to a project $\Pi_{\mathcal{S}_c}$ up to some scalar $c_D$.
    Therefore, using the stabiliser formalism, we can expand $D^I (D^I)^\dagger$: 
    \todo[inline]{Is this correct?}
    \begin{align*}
        \sum_{M \in valid_D}P_M D^I (D^I)^\dagger P_M = \sum_{M \in valid_D} P_M \left(\frac{c_D}{|\mathcal{S}_c|} \sum_{S \in \mathcal{S}_c} S\right) P_M = \frac{c_D}{|\mathcal{S}_c|} \sum_{S \in \mathcal{S}_c} \sum_{M \in valid_D} P_M S P_M
    \end{align*}
    $valid_D$ is a group and, by assumption, for every generator $S$ of $\mathcal{S}_c$ there exists a $M_S \in valid_D$ such that $P_{M_S}$ exactly anticommutes with $S$ and commutes with all other generators. 
    Thus, we know that for each $S \not= I$ there must be equally many $M \in valid_D$ such that $P_M$ and $S$ commute as there are $M$ such that they anticommute. 
    We can simply consider the two disjoint sets of values in $valid_D$ that respectively commute or anticommute with $S$ and observe that $M_S$ must create a bijection between those two sets. 
    Therefore, for all $S \not= I$, $\sum_{M \in valid_D} P_M S P_M$ must cancel out, leaving us with: 
    \begin{align*}
        \sum_{M \in \overline{\mathcal{P}_\mathcal{M}}} D^M (D^M)^\dagger
        & = \frac{c_D}{|\mathcal{S}_c|} \sum_{S \in \mathcal{S}_c} \sum_{M \in valid_D} P_M S P_M
          = \frac{c_D}{|\mathcal{S}_c|} \sum_{M \in valid_D} P_M I P_M \\
        & = \frac{c_D}{|\mathcal{S}_c|} \sum_{M \in valid_D} I P_M P_M
         = c_D\frac{|P_M|}{|\mathcal{S}_c|} I
    \end{align*}
    But then, for $c = \sqrt{\frac{|\mathcal{S}_c|}{c_D|P_M|}}$, we have $\sum_{M \in \overline{\mathcal{P}_\mathcal{M}}} cD^M (cD^M)^\dagger = I$.
\end{proof}

Now, we can prove: 
\begin{proposition}
    \label{prop:complete-measurements-circuit}
    Let $C$ be a quantum circuit and $D$ be the ZX diagram obtained from translating $C$ into a quantum circuit according to \autoref{fig:mappings}.
    Then, if we take the measurements in $D$ to be the obvious edge-flips as indicated by $C$, there exists a scalar $c$ such that $\mathcal M$ is complete for $cD$. 
\end{proposition}
\begin{proof}
We prove by induction on the number of gates that every ZX diagram derived from a circuit possesses a generating set of costabilizing Pauli webs $\mathcal{S}_c$ and a set of measurement flips ${M_{S_i}}$ satisfying the commutation relation $[M_{S_i}, S_j] = \delta_{ij}$.
For an identity circuit with zero gates, the set of costabilisers is empty, and the claim holds trivially.
Assume the claim holds for a circuit $C^k$ with $k$ gates with costabiliser generators $\mathcal{S}_c^k$ and respective measurements ${M_{S_i}^k}$.
If the $(k+1)$-th gate is unitary, the costabilizing group is unchanged, and the inductive hypothesis holds.
If the $(k+1)$-th gate is a measurement that measures an existing stabiliser of $C^k$, no new costabilisers are introduced, and the hypothesis remains satisfied.
If the $(k+1)$-th gate measures a logical operator of $C^k$, a new costabiliser $S_n$ is added to the generating set.
To ensure $S_n$ commutes with all previous measurement flips ${M_{S_i}^k}$, we update $S_n$ by multiplying it by any $S_i \in \mathcal{S}_c^k$ with which it anticommutes.
We define the new measurement flip $M_n$ as the Pauli operator corresponding to the outcome flip of the $(k+1)$-th gate.
By construction, $M_n$ anticommutes with $S_n$ but commutes with all $S_i \in \mathcal{S}_c^k$, as the latter are supported only on the previous $k$ gates.
The expanded set $\mathcal{S}_c^k \cup {S_n}$ and the corresponding measurements ${M_{S_i}^k} \cup {M_n}$ therefore satisfy the required conditions for \autoref{prop:measurement-completeness}.
This completes the inductive step and the proof.
\end{proof}

\subsection{Detectability of Faults}
In the main text, we defined a fault $F$ to be \emph{detectable} if $D^F = 0$.  
In this section, we show that this definition indeed captures the intended notion:  
if a fault is detectable according to the above criterion, then all valid measurement outcomes of the faulty circuit yield a nontrivial syndrome.  

First, we define and motivate a more suitable notion of detectability in the context of running ZX diagrams:

\begin{definition}[Detectability of faults]
    \label{def:generalisation-detectability}
    Let $F$ be a fault on $D$. 
    Then $F$ is detectable if and only if $valid_{D^F} \cap valid_D = \emptyset$. 
\end{definition}

The set $valid_D$ contains all measurement outcomes that could reasonably occur in the noise-free case for some input state.  
If a fault $F$ modifies this set so that every outcome possible on the faulty circuit is invalid for the original circuit, then any valid measurement observed on the faulty circuit certifies the presence of a fault.  
In other words, when $valid_{D^F} \cap valid_D = \emptyset$, the fault is necessarily detectable.  

We can now show:
\begin{proposition}
    Let $M \in valid_D$ and $F \in \overline{\mathcal{P}^{|E|}}$ such that $D^{MF} = 0$. 
    Then $F$ is detectable according to \autoref{def:generalisation-detectability}.
    Furthermore, if $F$ is detectable according to \autoref{def:generalisation-detectability}, then for all $M \in valid_D$ we have $D^{MF} = 0$.
\end{proposition}
\begin{proof}
    Suppose $M \in valid_D$ and $F \in \overline{\mathcal{P}^{|E|}}$ such that $D^{MF} = 0$. 
    We show that $F$ is detectable. 

    Let $M' \in valid_{D^F}$. 
    $D^{MF} = 0$ implies that $MF$ anticommutes with at least one detecting region \parencite{ruschCompletenessFault2025}. 
    As $M$ was assumed to be in $valid_D$ and must, therefore, commute with all detecting regions, this means that $F$ must anticommute with at least one detecting region.
    For some measurement outcome $M'$ to be valid in $D^F$ that means that $M'$ must anticommute with the same detection regions such that $M'F$ commutes with all detecting regions. 
    By \autoref{prop:valid-outcomes}, this means that $M'$ cannot be valid in $D$.
    As this holds for all $M \in valid_{D^F}$, we conclude
    \[
        valid_{D^F} \cap valid_D = \emptyset,
    \]
    and therefore $F$ is detectable.

    Now suppose $F$ is detectable.  
    Then we will show that for all $M \in valid_D$, we have $D^{MF} = 0$.
    As $F$ is detectable, all $M \in valid_D$ must be invalid in $D^F$. 
By \autoref{prop:valid-outcomes}, this means that $MF$ must anticommute with at least one detecting region. 
    Therefore, by \autoref{thm:detecting-region}, we must have $D^{MF} = 0$.

\end{proof}

Therefore, we have shown that the notion of detectability in the main paper is sufficient, meaning a fault is detectable according to the definition in the main body, if and only if it is detectable according to the definition proposed here. 

\subsection{Equivalence of Diagrams}
Running a diagram on some state results in two pieces of information: measurement outcomes sampled from some probability distribution and a new state.
We will define two diagrams to be equivalent if running one diagram gives the same information as if we had run the other.
For this, we need to take the measurement outcomes of the one diagram and translate them to equivalent measurement outcomes of the other diagram. 
Additionally, as we are considering Clifford diagrams, the output states may differ by a Pauli, which we can correct with a Pauli frame update.

Let $\mathscr{P}(S)$ denote the power set of $S$.
We have:
\begin{definition}
    Let $D_1$ and $D_2$ be ZX diagrams with measurement sets $\mathcal{M}_1, \mathcal{M}_2$. Then, we say $D_1$ can simulate $D_2$, if there exists a map $M_{D_1 \to D_2}: valid_{D_1} \to \mathscr{P}(valid_{D_1})$ and a set of Pauli operators $\{P_{M_1, M_2}\}_{M_1 \in valid_{D_1}, M_2 \in M_{D_1 \to D_2}(M_1)}$ such that given an input state $\psi$: 
    \begin{itemize}
        \item running $D_1$ on $\psi$ with measurement outcome $M_1$ and then uniformly sampling from $M_{D_1 \to D_2}(M_1)$ is like sampling from $\mathbb{P}_{D_2, \psi}$
        \item for all $M_1 \in valid_{D_1}$ and $M_2 \in M_{D_1 \to D_2}(M_1)$, we have: 
    \end{itemize}
    \[\tikzfig{appendix/simulation-statement}\]
    We say that $D_1$ and $D_2$ are equivalent if they can mutually simulate each other. 
    We write $D_1 \equiv D_2$.
\end{definition}

\subsubsection{Simulation Example}
To build some intuition on the definition above, we first explore an example of two equivalent diagrams; the identity and a teleportation:
\[\tikzfig{appendix/teleportation-equivalence}\]
To prove their equivalence, we show how they can be used to mutually simulate each other. 
We need to provide $M_{D_1 \to D_2}: valid_{D_1} \to \mathcal{P}(valid_{D_2})$ and Pauli operators $\{P_{M_1, M_2}\}_{M_1 \in valid_{D_1}, M_2 \in M_{D_1 \to D_2}(M_1)}$. 
In this example, we will simply provide them and prove mutual simulation. 
In \autoref{sec:simulation-examples}, we will show how to find $M_{D_1 \to D_2}$ and $\{P_{M_1, M_2}\}_{M_1 \in valid_{D_1}, M_2 \in M_{D_1 \to D_2}(M_1)}$ for more complicated simulation examples. 

We first show how to use the teleportation to simulate the identity. 
The identity has no measurements and therefore only has one possible measurement outcome; $I^{|E|}$.
The teleportation has one measurement: $(e, X)$ where $e$ is the edge before the single-legged red spider. 
It therefore has two possible measurement outcomes: $I, P_{(e, X)}$. 
For the sake of simplicity, we will refer to these to outcomes as $0, 1$, respectively.
We define $M_{D_t \to D_i}(M) = \{I^{|E|}\}$ for $M \in [0, 1]$.
In words, no matter what measurement outcome we get, to simulate the identity, we pretend that we did not do any measurement. 
Then, we define $P_{0, I^{|E|}} = I$ and $P_{1, I^{|E|}} = X$ to be the according Pauli corrections.
Now, when we run $D_t$ on some input state $\psi$ and then apply $M_{D_t \to D_i}$ to the measurement outcome, we always get the trivial outcome $I^{|E|}$.
This is exactly what we would get if we sampled from $\mathbb{P}_{D_i, \psi}$.
Additionally, if we apply the according correction, the resulting state will always be $\psi$. 
Therefore, we have used the teleportation to simulate the identity. 

We can similarly use the identity circuit to simulate the teleportation, so we do nothing but, up to a Pauli correction, we can pretend that we did the teleportation. 
We define $M_{D_t \to D_i}(I^{|E|}) = \{0, 1\}$ and  $P_{I^{|E|}, 0} = I$, $P_{I^{|E|}, 1} = X$.
Now, we can run $D_i$ on some input state $\psi$. 
To get a measurement outcome for $D_t$, we then uniformly sample from $M_{D_t \to D_i}(I^{|E|}) = \{0, 1\}$, i.e. we randomly pick $0$ or $1$. 
Based on that, we do the according Pauli correction. 
If we had run $D_t$ on $\psi$, the measurement outcome would be uniformly random, i.e. $\mathbb{P}_{D_t, \psi}(0) = \mathbb{P}_{D_t, \psi}(1) = 0.5$. 
In the simulation procedure where we uniformly sample from $\{0, 1\}$, we get the same probability distribution. 
Additionally, since we do the according Pauli correction, for each simulated measurement outcome, we also perform the same linear map. 
Thus, we have used the identity to simulate the teleportation. 

\subsubsection{Simulation Proof}
Building on the intuitions form the example above, we can finally show that our notion of equivalence in the main body implies mutual simulability, i.e.\@ implies that we could run either circuit and get the same outcomes as with the other circuit.

We have: 
\begin{theorem}[Equivalent ZX diagrams]
    \label{thm:equivalence}
    Let $D_1$ and $D_2$ be ZX diagrams with respective complete measurement outcomes $\mathcal M_1, \mathcal M_2$.
    Then if there exist a measurement outcome $M \in \mathcal M_1$ and $M' \in \mathcal M_2$, such that $D_1^{M} \propto D_2^{M'} \not= 0$ then $D_1$ can simulate $D_2$.
\end{theorem}
\begin{proof}
    \todo[inline]{This is the proof, I am currently the least sure about.}
    To show that $D_1$ can simulate $D_2$, we first define $M_{D_1 \to D_2}$ and $P_{M_1, M_2}$ before showing that they satisfy the necessary conditions. 
    
    As $D_1^{M_1} \propto D_2^{M_2}$, there must exist some $c$ such that $D_1^{M_1} = c D_2^{M_2}$. 
    This means that the two diagrams must have the same stabilisers.
    For $M_1 \in valid_{D_1}$, we define $M_{D_1 \to D_2}(M_1)$ as the set of all $M_2 \in valid_{D_2}$ such that $M_1$ and $M_2$ anticommute with the same costabilisers. 
    By \autoref{prop:measurement-completeness}, we know that for each $M_1$, there must exist at least one $M_2$ that anticommutes with the same stabilisers.
    We then define $P_{M_1, M_2}$ to consist of exactly those destabilisers on the output of $D_1$, such that $P_{M_1, M_2} D_1^{M_1}$ and $D_2^{M_2}$ flip the same stabilisers and logicals. 
    By stabiliser theory, we know that such a $P_{M_1, M_2}$ must always exist. 
    But then, as $P_{M_1, M_2} D_1^{M_1}$ and $D_2^{M_2}$ now flip exactly the same co-stabilisers, stabiliser and logicals, we must have $P_{M_1, M_2} D_1^{M_1} = cD_2^{M_2}$

    \todo[inline]{There is something about global scalars that I am not yet sure about.}

    For $D_1$ to simulate $D_2$, two conditions have to hold; (1) sampling $M$ from $\mathbb{P}_{D_1, \psi}$ and then sampling uniformly from $M_{D_1 \to D_2}(M)$ is like sampling from $M_{D_1 \to D_2}$ and (2) the resulting output state after correction is the same. 
    The latter is naturally satisfied as we chose $P_{M_1, M_2}$ such that $P_{M_1, M_2} D_1^{M} = c D_2^{M_2}$. 
    Thus, it remains to be shown that the first condition is satisfied as well. 

    Let $M \in valid_{D_1}$. 
    We will consider the equivalence class $[M]$ of all values in $valid_{D_1}$ that flip the same costabilisers as $M$. 
    First, we show that all values $[M]$ are equally likely. 
    Let $\psi$ be a normalised input state to $D_1$. 
    Then, we have:  
    \[\resizebox{\textwidth}{!}{\tikzfig{appendix/equally-likely-proof-2}}\]
    where we can always find a $P$ such that $P D^{M_1} = D^{M_2}$ by the same logic as above. 
    Thus, we know that 
    \[\mathbb{P}_{D_1, \psi}(M_1) = \mathbb{P}_{D_1, \psi}([M_1]) \times \frac{1}{|[M_1]|}\]

    $D_1$ and $D_2$ have the same stabilisers, and, as we assumed $\mathcal M_1, \mathcal M_2$ to be complete, by \autoref{prop:measurement-completeness}, we know that for each generator of the costabilisers there exists at least one measurement such that exactly that costabiliser is flipped. 
    Thus, for all equivalence classes $[M_1]$ on $D_1$, there exists an equivalence $[M_2]$ on $D_2$ that flips exactly the same costabilisers. 
    Furthermore, as both measurement sets are assumed to be complete and the diagrams measure exactly the same costabilisers, we know that $\sum_{M \in M_1} \mathbb{P}_{D_1, \psi}(M) = \mathbb{P}_{D_1, \psi}([M_1]) = \mathbb{P}_{D_2, \psi}([M_2]) = \sum_{M \in M_2} \mathbb{P}_{D_2, \psi}(M)$.
    \todo[inline]{@Aleks, this seems just true. Do I need to justify it more?}
    We now have for all $M_2 \in valid_{D_2}$:
    \begin{align*}
        \mathbb{P}_{sim}(M_2) = \mathbb{P}_{D_1, \psi}([M_1]) \times \frac{1}{|[M_2]|} 
        = \mathbb{P}_{D_2, \psi}([M_2]) \times \frac{1}{|[M_2]|}
        = \mathbb{P}_{D_2, \psi}(M_2)
    \end{align*}
    Thereby proving our claim.
\end{proof}

In the main body, we show equivalences of linear maps up to global scalar while post-selecting on some valid measurement outcome. 
We have just shown that if we treat two diagrams as equal in the main body, they must be able to simulate each other, assuming that we provide complete measurement outcomes.
By \autoref{prop:complete-measurements-circuit}, we know that ZX diagrams that represent quantum circuits have obvious complete measurement outcomes. 
Thus, we have proven that the equivalence in the main body is a sufficient condition for mutual simulation.

We can observe that the opposite is not true; if $D_1$ can simulate $D_2$, there may not exist measurement outcomes such that the two circuits implement the same linear map. 
A simple example for two circuits that can simulate each other but would not be treated as equivalent in the main body are unitary Pauli rotations. 
For example: 
\[\tikzfig{appendix/simulation-examples/simple-counter-example}\]
These circuits are clearly equivalent; $M_{D_1 \to D_2}$ is trivial, mapping $I^{|E|}$ to $\{I^{|E|}\}$ and $P_{I^{|E|}, I^{|E|}} = Z$. 
However, as there are no measurement outcomes, there clearly exists no measurement outcomes that make the two circuits implement the same linear map --- they only do so up to a Pauli correction. 
Therefore, while they can simulate each other, in the main body, we would not treat them as equivalent. 
However, we can state: 
\begin{proposition}
    Let $D_1 \equiv D_2$, then there exists measurement outcomes $M_1, M_2$ and a Pauli correction $P$ such that $P D_1^{M_1} = D_2^{M_2}$.
    Let $D_1 \equiv D_2$, then there exists measurement outcomes $M_1, M_2$ and a Pauli correction $P$ such that $P D_1^{M_1} = D_2^{M_2}$.
\end{proposition}
\begin{proof}
    This trivially follows from $D_1$ being able to simulate $D_2$.
    This trivially follows from $D_1$ being able to simulate $D_2$.
\end{proof}

As such, the equivalence in the main body is a sufficient condition for equivalence in the sense of mutual simulation. 
In particular, it furthermore requires that $I \in M_{D_1 \to D_2}(I)$ and that $P_{I, I} = I$. 
However, if two diagrams can simulate each other, there always exists a set of measurement outcomes and Pauli corrections such that the underlying diagrams implement the same linear map. 
Therefore, even though the notion of equivalence in the main body is slightly more restrictive than mutual simulation, it is only so up to a Pauli correction.

\subsection{More Simulation Examples}
\label{sec:simulation-examples}
In this section, we will show how to derive $M_{D_1 \to D_2}$ and $P_{M_1, M_2}$ from two ZX diagrams that implement the same linear map. 
For this, we start with $D_1$, adding the potential edge flips as parameterised spiders.
Then we rewrite $D_1$ into $D_2$, followed by some Pauli corrections.
From the resulting diagram, we can read off the desired values.

\subsubsection{Example 1: Shor-style Syndrome Extraction}
The first example we consider is Shor's implementation of a weight-four $X$ measurement. 
It results in four measurement outcomes that together determine the outcome of the stabiliser measurement. 
We have: 
\[\tikzfig{appendix/simulation-examples/shor-to-spec}\]
We can now read off that $M_{D_{shor} \to D_{spec}}(k_1k_2k_3k_4) = \{k\}$ where $k = k_1 \oplus k_2 \oplus k_3 \oplus k_4$. 
In practice, this means that the measurement outcome of the specification can be calculated by taking the parity of the four destructive measurements. 
Furthermore, we can see that no Pauli frame updates are necessary. 

However, we can also go the other way around; we can run the specification to simulate the Shor-style syndrome extraction: 
\[\tikzfig{appendix/simulation-examples/spec-is-shor}\]
Now, $M_{D_{spec} \to D_{shor}}(k) = \{k_1k_2k_3k_4\}$ where $k_1 \oplus k_2 \oplus k_3 \oplus k_4 = k$. 
So $k$ is mapped to the set of measurement outcomes $k_1k_2k_3k_4$ whose parity is $k$. 
Thus, to simulate Shor-style syndrome extraction using the specification, once we measured the stabiliser, we sample some combination of $k_i$'s such that their parity is $k$.
Once again, no Pauli frame corrections are necessary. 

\subsubsection{Example 2: Optimised Shor-style Syndrome Extraction}
As a slightly more complicated example, we can consider the optimised implementation of Shor's syndrome extraction. 
As it includes the cat-like linear map, it has more measurements and does need Pauli frame updates: 
\[\tikzfig{appendix/simulation-examples/optimised-shor-is-spec}\]
Thus, $M_{D_{opt.-shor} \to D_{spec}}(k_1k_2k_3k_4) = \{k\}$ where $k = k_1 \oplus k_2$ and $P_{k_1k_2k_3k_4, k} = Z^{k_3} \otimes I \otimes Z^{k_4} \otimes I$.
Furthermore, we see the free-floating green spider with phase $(k_3 \oplus k_4) \pi$. 
This reflects the fact that $D_{opt.-shor}$ has a detecting region that covers measurements three and four, meaning that their parity is predetermined in all valid measurement outcomes. 
For the diagram to be non-zero, $k_3 \oplus k_4 = 0$ must be satisfied. 

Once again, we can also go the other way:
\[\tikzfig{appendix/simulation-examples/spec-is-optimised-shor}\]
We have $M_{D_{spec} \to D_{shor}}(k) = \{k_1k_2k_3k_3\}_{k = k_1 \oplus k_2}$ and $P_{k, k_1k_2k_3k_4} = Z^{k_3} \otimes I \otimes Z^{k_4} \otimes I$.
Thus, to simulate the optimised Shor-style syndrome extraction, using the specification, once measuring the stabiliser, we sample values $k_1$ and $k_2$ such that their parity is $k$, and then we sample $k_3$ to indicate the green projective measurements. 
The fact that we only sample one value for $k_3$ and $k_4$ once again reflects that in all $valid_{D_{opt.-shor}}$, we have $k_3 = k_4$.

\subsubsection{On the Limits of Simulation}
It is essential to remark that simulation is for the fault-free execution of diagrams. 
If faults occur, mutual simulation becomes more complicated. 
In particular, noisy simulation has to be separated into two steps; (1) decoding and (2) noise-free simulation. 

We can view decoding as, given a syndrome, identifying the most likely edge flip with that syndrome such that applying the edge flip once again gives us a syndrome-free circuit.
Once we have decoded, we can once more apply the simulation procedure outlined above, which maps valid measurement outcomes to valid measurement outcomes.
For noise-free simulation, we can use the one process and linear classical compute to create the effect of the other process. 
It would be desirable for something similar to be possible for decoding; given an efficient decoder for one process, efficiently decode the other. 
This is, however, not generally possible \parencite{schweikart}. 
Fault-equivalent rewrites can introduce and remove detecting regions, fundamentally changing the decoding problem. 
Therefore, in general, we can not expect any guarantees for the decoding problem of one circuit given the decoding problem for an equivalent one. 

To simulate one circuit in a noisy setting, given another, we have to tackle the decoding problem from scratch. 
There are settings in which it is relatively easy to calculate the updated decoder \parencite{schweikart, ultra-low-overhead}, however, to the best of our knowledge, this is not possible in general.
Thus, to run one circuit instead of the other, in the noisy setting, one has to recompute the decoding problem from scratch, e.g., using Pauli webs \parencite{ruschCompletenessFault2025}, and create a completely new decoder.
Once a given noisy instance is decoded, one can use the simulation above.

\subsection{Fault Equivalence}
The final definition, we have to prove correct is fault equivalence. 
We have shown that we can think about equivalent circuits as mutually simulating each other, meaning that we run one circuit but, with a little bit of post-processing, we get the same information as if we had run the other circuit. 
We will now show that if two circuits are fault-equivalent, then if we run one circuit under noise, for any fault that can occur, there is an equivalent fault that could have occurred on the other circuit to give the same results. 

\begin{definition}[Fault-equivalence]
    \label{def:fault-equivalent-non-determinisitic}
    Let $D_1$ and $D_2$ be equivalent diagrams with respective simulation information $M_{D_1 \to D_2}$, $\{P_{M_1, M_2}\}$ and $M_{D_2 \to D_1}$, $\{P_{M_2, M_1}\}$.
    Then we say that $D_1$ is fault-equivalent to $D_2$, if for every fault $F_1 \in valid_{D_1}$, there exists a fault $F_2 \in valid_{D_2}$ such that $wt(F_2) \leq wt(F_1)$ and for all input states $\psi$, we have: 
    \begin{itemize}
        \item running $D_1^{F_1}$ on $\psi$ with measurement outcome $M_1$ and then uniformly sampling from $M_{D_1 \to D_2}(M_1)$ is like sampling from $\mathbb{P}_{D_2^{F_2}, \psi}$
        \item for all $M_1 \in valid_{D_1}$ and $M_2 \in M_{D_1 \to D_2}(M_1)$, we have: 
    \end{itemize}
    \[\tikzfig{appendix/faulty-simulation-statement}\]
    and the same holds for all $F_2 \in valid_{D_2}$.
\end{definition}

\begin{proposition}
    Let $D_1$ and $D_2$ be ZX diagrams with respective complete measurement outcomes $\mathcal M_1, \mathcal M_2$ and noise models $\mathcal{F}_1, \mathcal{F}_2$.
    Then, if $D_1$ is fault-equivalent to $D_2$ according to \autoref{def:fault-equivalence}, $D_1$ is also fault equivalent to $D_2$ according to \autoref{def:fault-equivalent-non-determinisitic}.
\end{proposition}
\begin{proof}
    ASs$D_1$ and $D_2$ are fault equivalent according to \autoref{def:fault-equivalence}, we know that $D_1^I = D_2^I$, as the trivial fault is the only fault of weight $0$ on either circuit. 
    Thus, for $F_1 = I$, there must exist a fault of weight $0$ on $D_2$ such that $D_1^I = D_2^F$.

    But then, by \autoref{thm:equivalence}, we know that there exits $M_{D_1 \to D_2}$, $\{P_{M_1, M_2}\}$ and $M_{D_2 \to D_1}$, $\{P_{M_2, M_1}\}$ such that $D_1$ and $D_2$ can respectively simulate each other. 

    Let $F_1 \in valid_{D_1}$. 
    This means that $F_1$ must be undetectable.
    Thus, according to $D_1$ and $D_2$ being fault equivalent, there must exist a fault $F_2$ on $D_2$ such that $D_1^{F_1} = D_2^{F_2}$ and $wt(F_2) \leq wt(F_1)$. 
    As $D_1^{F_1} = D_2^{F_2}$, this means that $F_2$ must also be undetectable and thus $F_2 \in valid_{D_2}$. 

    Finally, we will show that running $D_1^{F_1}$ with corrections $M_{D_1 \to D_2}$ and $\{P_{M_1, M_2}\}$ is like running $D_2^{F_2}$. 
    By \textcite{ruschCompletenessFault2025}, we know that for all undetectable $F_1$, there exist $P_I^{F_1}$ and $P_O^{F_1}$ such that: 
    \[\tikzfig{appendix/pushing-out}\]
    Furthermore, as $D_1^{F_1} = D_2^{F_2}$, $P_I^{F_1}$ and $P_O^{F_1}$ must further satisfy the same for $D_2$:
    \[\tikzfig{appendix/pushing-out-D2}\]

    But then, for all normalised input states $\psi$, we can observe that: 
    \[\tikzfig{appendix/noisy-sampling-distribution}\]
    Analogously, it follows that $\mathbb{P}_{D_2^{F_2}, \psi}(M_2)$ = $\mathbb{P}_{D_2,P_I^{F_1} \psi}(M_2)$.
    But as $P_I^{F_1} \psi$ is still a normalised input state, by $D_1$ being able to simulate $D_2$, we now know that sampling $M_1$ from $\mathbb{P}_{D_1^{F_1}, \psi}$ and then uniformly sampling from $M_{D_1 \to D_2}(M_1)$ is like sampling from $\mathbb{P}_{D_2^{F_2}, \psi}$.

    Finally, we can show that for all $M_1 \in valid_{D_1}$ and $M_2 \in M_{D_1 \to D_2}(M_1)$, we have: 
    \[\tikzfig{appendix/faulty-simulation-statement}\]
    We have: 
    \[\tikzfig{appendix/faulty-simulation-map-proof}\]
    The second step follows from Paulis either commuting or anticommuting.
    The third step follows form $D_1$ simulating $D_2$ and the final step is the reverse of the first step, however, now on $D_2$.
\end{proof}
