# Supplementary material for: Fault Tolerance by Construction
Source: arXiv:2506.17181 source file (2026-03-31)
Supplement: Supplementary file 6 [file 06-measurement-outcomes.tex]

\section{Measurement Outcomes in ZX Diagrams}
In the main body, we treat ZX diagrams as linear maps.
In practice, ZX diagrams implement non-deterministic computations.
In this appendix, we formalise the role of measurements in ZX diagrams.
Using this framework, we redefine three notions that are essential for our paper: detectability of faults, equivalence of diagrams, and fault equivalence of diagrams.
We then show that the definitions used in the main body are satisfied if and only if their counterparts for non-deterministic computations are satisfied.
This result justifies the simplified treatment of ZX diagrams as linear maps adopted in the main body.
The key takeaway is that measurements need not be tracked explicitly during derivations.

Furthermore, we provide the necessary tools to replace one Clifford subcircuit with another and give ways of interpreting the corresponding measurement outcomes.
Importantly, in the noise-free case, we never need any post-selection for one equivalent ZX diagram to take the place of another.

Before proceeding, we introduce some additional terminology.
In \autoref{sec:detection-regions}, we introduced Pauli webs and highlighted the special role of detecting regions, that is, Pauli webs that act trivially on the boundary edges.
For the treatment of measurement outcomes, however, it is necessary to consider all Pauli webs.
We therefore introduce the following terminology:
\begin{definition}[Stabilising, costabilising, and logical Pauli webs]
    Let $D$ be a ZX diagram.  
    A Pauli web $P \in \overline{\mathcal{P}^{|E|}}$ is called
    \begin{itemize}
        \item a \emph{stabilising Pauli web} if it acts trivially on all input edges,
        \item a \emph{costabilising Pauli web} if it acts trivially on all output edges,
        \item a \emph{logical Pauli web} if it acts nontrivially on both inputs and outputs.
    \end{itemize}
\end{definition}
Furthermore, we consider costabilisers to be Paulis that are stabilised on the input, meaning precomposing a diagram with some Pauli $P$ does not change the underlying linear map. 
As such, they are the analogue to stabilisers which are defined on the outputs.

\textcite{rodatzFloquetifyingStabiliser2024} show the relationship between Pauli webs and stabilisers, costabilisers and logicals. 
In particular, for every stabiliser of some diagram $D$, there exists a corresponding Pauli web that has the same action on the output wires. 
Similarly, the action of every stabilising Pauli web corresponds to stabilisers of $D$. 

\subsection{Running ZX Diagrams}
In the main body, we treat ZX diagrams as static, linear maps. 
However, in practice, they represent quantum computations that are run on quantum computers. 
For a given input, running a computation results in classical measurement outcomes, sampled from some probability distribution, and results in a new state.

First, we define: 
\begin{definition}[Measurement outcome]
    Let $D$ be a ZX diagram with edges $E$. 
    A measurement outcome on $D$ is an element in $\overline{\mathcal{P}^{|E|}}$.
\end{definition}

Usually, when translating between measurements on quantum circuits and ZX diagrams, parameterised spiders are used. 
For example a single, destructive $Z$ measurement could be represented as follows: 
\[\tikzfig{appendix/measurement-outcomes}\]
where the Boolean parameter $k$ indicates the measurement outcome. 
Instead, we propose to unfuse the parameterised spider and view it as an edge flip on the edge before the measurement: 
\[\tikzfig{appendix/unfuse-measurement}\]
where the Boolean parameter $k$ indicates the measurement outcome. 
Thus, flipping a measurement is the same as having an edge flip just before the measurement. 
This observation will later allow us to use various results about edge flips to reason about measurement outcomes.

One key difference between quantum circuits and ZX diagrams is that we do not attribute a specific role to specific spiders. 
Therefore, we simply allow measurement outcomes to act on all edges, not just dedicated ones. 
We will later relate this back to measurement outcomes on quantum circuits. 

We can now define:
\begin{definition}[Running a ZX diagram without noise]
    Given a ZX diagram $D$ and a normalised input state $\psi$, running $D$ on $\psi$ results in two pieces of information: 
    \begin{enumerate}
      \item a measurement outcome $M \in \overline{\mathcal{P}^{|E|}}$ sampled from a probability distribution $\mathbb{P}_{D, \psi}$
      \item a new state $D^M \ket{\psi}$ which is conditions on the measurement outcome
    \end{enumerate}
    where $\mathbb{P}_{D, \psi}(M)$ for $M \in \overline{\mathcal{P}^{|E|}}$ is given by the Born rule as: 
    \[\tikzfig{appendix/born-rule}\]
\end{definition}

Running a ZX diagram with noise consists of running a ZX diagram without noise as outlined above and then sampling a fault from some distribution of our faults as determined by the noise model. 
The resulting measurement outcome would then be $FM$. 
The task of decoding then consists of identifying the $F$ component of the measurement outcome.

Next, we define: 
\begin{definition}
    Let $D$ be a ZX diagram.
    We say a measurement outcome $M \in \overline{\mathcal{P}^{|E|}}$ is valid, if there exists an input state $\psi$, such that $\mathbb{P}_{D, \psi}(M) \not= 0$. 
    We call the set of all valid measurement outcomes $valid_D \subseteq \overline{\mathcal{P}^{|E|}}$. 
\end{definition}

For example, consider two consecutive $ZZ$ measurements. 
Certain outcome sequences are not physically consistent in the absence of noise. 
On quantum circuits, this corresponds to the fact that, although two measurements are performed, only the outcome pairs $00$ or $11$ should occur. 
If instead $01$ or $10$ is observed, this indicates that a fault must have occurred, since these outcomes are not valid without errors.
Analogously, on the ZX diagram, we would not expect to observe an odd number of $X$ or $Y$ edge flips in the detecting region formed by the two measurements.

We can characterise the set of valid measurement outcomes further. 
To study the effect of an edge flip $M$ on a diagram $D$, we can first observe that $D^I$ and $D^M$ must have the same stabilising Pauli webs \parencite{ruschCompletenessFault2025}.
The only difference between the two linear maps can therefore be whether they live in the $+1$ or $-1$ eigenspace of the corresponding stabilisers. 
Or, in other words, the effect of edge-flips is fully described by the Pauli webs they flip.

As measurements are special kinds of edge-flips, we can have a closer look at the potential effects of measurements: 
\begin{proposition}
    \label{prop:valid-outcomes}
    A measurement outcome is valid if and only if it commutes with all detecting regions.
\end{proposition}
\begin{proof}
    Let $M$ be a measurement outcome that anticommutes with a detecting region.  
    Then, by \autoref{thm:detecting-region}, we have $D^M = 0$.  
    This implies that the probability of observing $M$ is zero for every input state.  
    Hence, $M$ cannot be valid.

    Let $M$ be a measurement outcome that commutes with all detecting regions. 
    Then take any normalised state $\psi$ that lives in the $+1$ eigenspace of all the costabilisers of $D^M$. 
    Now, $\bra{\psi} D^M (D^M)^\dagger \ket{\psi}$ has no violated detecting region. 
    Therefore, it must be non-zero \parencite{ruschCompletenessFault2025} and thus, $M$ is valid. 
\end{proof}

\subsection{Detectability of Faults}
In the main text, we defined a fault $F$ to be \emph{detectable} if $D^F = 0$.  
In this section, we show that this definition indeed captures the intended notion:  
if a fault is detectable according to the above criterion, then all valid measurement outcomes of the faulty circuit yield a nontrivial syndrome.  

First, we define and motivate a more suitable notion of detectability in the context of running ZX diagrams:
\begin{definition}[Detectability of faults]
    \label{def:generalisation-detectability}
    Let $F$ be a fault on $D$. 
    Then $F$ is detectable if and only if $valid_{D^F} \cap valid_D = \emptyset$. 
\end{definition}

The set $valid_D$ contains all measurement outcomes that could reasonably occur in the noise-free case for some input state.  
If a fault $F$ modifies this set so that every outcome possible on the faulty circuit is invalid for the original circuit, then any valid measurement observed on the faulty circuit certifies the presence of a fault.  
In other words, when $valid_{D^F} \cap valid_D = \emptyset$, the fault is necessarily detectable.  

We can now show:
\begin{proposition}
    Let $F \in \overline{\mathcal{P}^{|E|}}$.  
    Then $F$ is detectable according to \autoref{def:generalisation-detectability} if and only if $D^F = 0$.
\end{proposition}
\begin{proof}
    ($\Rightarrow$) Suppose $F$ is detectable according to \autoref{def:generalisation-detectability}.  
    By \autoref{prop:valid-outcomes}, this means that $F$ must anticommute with at least one detecting region.  
    Therefore, by \autoref{thm:detecting-region}, we have $D^F = 0$.

    ($\Leftarrow$) Suppose $F \in \overline{\mathcal{P}^{|E|}}$ such that $D^{F} = 0$ and $M \in valid_{D}$. 
    $D^{F} = 0$ implies that $F$ anticommutes with at least one detecting region \parencite{ruschCompletenessFault2025}. 
    But as $M \in valid_{D}$, $M$ must commute with all detecting regions. 
    Therefore, $FM$ must anticommute with at least one detecting region and, as such, $M$ cannot be in $valid_{D^F}$.
    As this holds for all $M \in valid_{D}$, we conclude
    \[
        valid_{D^F} \cap valid_D = \emptyset,
    \]
    and therefore $F$ is detectable.
\end{proof}

Therefore, we have shown that the notion of detectability in the main paper is sufficient, meaning a fault is detectable according to the definition in the main body, if and only if it is detectable according to the definition proposed here. 

\subsection{Equivalence of Diagrams}
Running a diagram on some state results in two pieces of information: measurement outcomes sampled from some probability distribution and a new state.
We will show that if two diagrams represent the same linear map, running one gives no more information than running the other. 
For this, we need to take the measurement outcomes of the one diagram and translate them to equivalent measurement outcomes of the other diagram. 
Additionally, as we are considering Clifford diagrams, the output states may differ by a Pauli, which we can correct by a Pauli correction.

As observed in \cite{ruschCompletenessFault2025}, edge flips can fully be described by the Pauli webs they anti-commute with. 
Here, we are mostly interested in the costabilising Pauli webs a measurement flips. 
Let $\mathscr{P}(\mathcal{S})$ denote the power set of $\mathcal{S}$.
\begin{definition}[Branch function]
    Let $D$ be a ZX diagram with costabilisers $c\mathcal{S}$. 
    We define the branch function $\mathscr{B}_D: \overline{\mathcal{P}^{|E|}} \to \mathscr{P}(c\mathcal{S})$ for some $M \in \overline{\mathcal{P}^{|E|}}$ to be the set of all costabilisers $M$ flips.   
    Furthermore, we define $\mathscr{B}^{-1}_D: \mathscr{P}(c\mathcal{S}) \to \overline{\mathcal{P}^{|E|}}$ to be the function that maps all powersets of $c\mathcal{S}$ to the set of measurement outcomes that exactly anticommute with that subset of $c\mathcal{S}$.
\end{definition}

To figure out the costabilisers $M$ flips, we can take any of the costabilising Pauli webs associated with some stabiliser and take their commutation relationship with $M$. 
By linearity, this implies that branches can be fully characterised by choosing a basis of costabilisers and considering the commutation relationship between each measurement outcome and that basis element. 
However, for the sakes of simplicity, we will avoid fixing a basis. 

We can now define an equivalence relationship on the measurement outcomes, where we consider two measurement to be equivalent, if they live in the same branch. 
As we only expect to see valid measurement outcomes, we will focus on those:
\begin{definition}
    Let $M_1, M_2$ be valid measurement on some ZX diagram $D$. 
    Then we say $M_1$ and $M_2$ are branch-equivalent, written $M_1 \equiv_{\mathscr{B}_D} M_2$ if and only if $\mathscr{B}_D(M_1) = \mathscr{B}_D(M_2)$.
    We write $[M_1]_{\mathscr{B}_D}$ to indicate the branch-equivalence class of $M_1$.
\end{definition}

We can observe that, if two measurement outcomes are branch-equivalent, then they implement the same linear map up to a Pauli correction on the outputs:
\begin{proposition}
    \label{prop:pauli-correction}
    Let $M$ be valid measurement on some ZX diagram $D$.
    Then there exists a Paulis $P_i^{\mathscr{B}_D(M)}, P_o^{M}$ such that: 
    \[\tikzfig{appendix/pushing-out-statement}\]
    where $P_i^{\mathscr{B}_D(M)}$ only depends on the branch of $M$. 
\end{proposition}
\begin{proof}
    From \cite{ruschCompletenessFault2025}, we know that two edge flips create the exact same linear map, if and only if they anticommute with the same Pauli webs. 
    As $M$ was assumed to be valid, it must commute with all detecting regions. 
    But then, by stabiliser theory, we can find the destabilisers on the boundary that flip exactly the same Pauli webs as $M$. 
    Furthermore, we can choose $P_i^{\mathscr{B}_D(M)}$ to flip exactly the same costabilisers as $M$ and choose $P_o^{M}$ to flip the remaining logicals and stabilisers. 
    As such $P_i^{\mathscr{B}_D(M)}$ only depends on the costabilisers $M$ flips, i.e.\@ the branch of $M$. 
\end{proof}

Furthermore, we can observe that two branch-equivalent outcomes are equally likely:
\begin{proposition}
    \label{prop:equally-likely}
    Let $M_1, M_2$ be valid measurement on some ZX diagram $D$ such that $M_1 \equiv_{\mathscr{B}_D} M_2$.
    Then for all states $\psi$, we have $\mathbb{P}_{D, \psi}(M_1) = \mathbb{P}_{D, \psi}(M_2)$.
\end{proposition}
\begin{proof}
    By \autoref{prop:pauli-correction}, we know that there must exist some Pauli $P_{M_1, M_2}$ such that $P_{M_1, M_2} D^{M_1} = D^{M_2}$. 
    But then, we have:
    \[\resizebox{\textwidth}{!}{\tikzfig{appendix/equally-likely-proof-2}}\]
    And therefore, we must have $\mathbb{P}_{D, \psi}(M_1) = \mathbb{P}_{D, \psi}(M_2)$.
\end{proof}

Finally, we observe that all equivalence classes are equally large: 
\begin{proposition}
    Let $M_1, M_2$ be valid measurement on some ZX diagram $D$. 
    Then $|[M_1]_{\mathscr{B}_D}| = |[M_2]_{\mathscr{B}_D}|$.
\end{proposition}
\begin{proof}
    Let $c\mathcal{S} = \{cS_1, \dots, cS_n\}$ be a generating set for all costabilisers of $D$. 
    Then $M_1$ and $M_2$ flips some set of these. 
    Let $cS_{i_1}, \dots cS_{i_k}$ be the costabilisers, that $M_1$ and $M_2$ flip differently. 
    Then, by stabiliser theory, we know that there must exists a destabiliser on the input of $D$ that anticommutes with exactly these costabilisers. 
    We can read this destabiliser as an edge flip $E$. 
    But then $E$ is a bijection between $[M_1]_{\mathscr{B}_D}$ and $[M_2]_{\mathscr{B}_D}$ that maps every element in $[M_1]_{\mathscr{B}_D}$ to an element in $[M_2]_{\mathscr{B}_D}$ and vice versa. 
    Therefore, the two equivalence classes must be of equal size. 
\end{proof}

Finally, we can state: 
\begin{theorem}[Mutual simulation]
    \label{thm:mutual-simulation}
    Let $D_1, D_2$ be ZX diagrams such that $D_1^I \propto D_2^I$. 
    Then, for all input states $\psi$, sampling $M_1$ from $\mathbb{P}_{D_1, \psi}$ and then uniformly sampling $M_2$ from $\mathscr{B}^{-1}_{D_2}(\mathscr{B}_{D_1}(M_1))$ is like sampling from $\mathbb{P}_{D_2, \psi}$.
    Furthermore, for all $M_2$ obtained in that way, we can find a $P_{M_1, M_2}$ such that $P_{M_1, M_2} D_1^{M_1} = D_2^{M_2}$.
\end{theorem}
\begin{proof}
    As $D_1 \propto D_2$, they have the same set of costabilisers. 

    First, we will show that for all $cS \subseteq c\mathcal{S}$, we have that 
    \[\sum_{M \in \overline{\mathcal{P}^{|E_1|}} \text{ with } \mathscr{B}_{D_1}(M) = cS} \mathbb{P}_{D_1, \psi}(M) = \sum_{M \in \overline{\mathcal{P}^{|E_2|}} \text{ with } \mathscr{B}_{D_2}(M) = cS} \mathbb{P}_{D_2, \psi}(M)\]
    Meaning that the probability of seeing some branch on $D_1$ must be the same as seeing that same branch on $D_2$. 

    We will show this by contradiction. 
    Without loss of generality, let us assume that for some branch $cS$, we have:
    \[\sum_{M \in \overline{\mathcal{P}^{|E_1|}} \text{ with } \mathscr{B}_{D_1}(M) = cS} \mathbb{P}_{D_1, \psi}(M) > \sum_{M \in \overline{\mathcal{P}^{|E_2|}} \text{ with } \mathscr{B}_{D_2}(M) = cS} \mathbb{P}_{D_2, \psi}(M)\]

    Then we can show that for all other branches $cS'$, we also have:
    \[\sum_{M \in \overline{\mathcal{P}^{|E_1|}} \text{ with } \mathscr{B}_{D_1}(M) = cS'} \mathbb{P}_{D_1, \psi}(M) \geq \sum_{M \in \overline{\mathcal{P}^{|E_2|}} \text{ with } \mathscr{B}_{D_2}(M) = cS'} \mathbb{P}_{D_2, \psi}(M)\]
    This will lead to a contradiction, as we assume both probability distributions to sum to one and we have just shown that one is strictly larger than the other.

    With, we observe that branches $cS'$ have valid measurement outcomes on $D_1$ if and only if they have valid measurement outcomes on $D_2$. 
    This follows from \autoref{prop:pauli-correction}, which allows us to push all valid measurement outcomes to the boundary. 
    But as both diagrams have the same boundary, for all valid measurement outcomes on one diagram, there must exist at least one equal measurement outcome on the other diagram.

    For all branches without valid measurement outcomes the probability of getting that branch is zero, so the inequality above trivially holds.

    For all other branches, we have: 
    \begin{align*}
        &\sum_{M \in \overline{\mathcal{P}^{|E_1|}} \text{ with } \mathscr{B}_{D_1}(M) = cS} \mathbb{P}_{D_1, \psi}(M) \\
        &= \tikzfig{appendix/simulation-proof/step1} \\[1cm]
        &= \tikzfig{appendix/simulation-proof/step2} \\[1cm]
        &= \tikzfig{appendix/simulation-proof/step3}
    \end{align*}
    \todo[inline]{complete}

    As $D_1 \propto D_2$, there exists some $c$ such that $D_1 = cD_2$.

    But then, as we have previously shown that all $M$ in the same branch are equally likely, we have: 
    \begin{align*}
        \mathbb{P}_{sim}(M_2) &= \sum_{M_1 \in \overline{\mathcal{P}^{|E_1|}} \text{ with } \mathscr{B}_{D_1}(M_1) = \mathscr{B}_{D_2}(M_2)} \mathbb{P}_{D_1, \psi}(M_1) \times \frac{1}{|[M_2]|}\\
        &= \sum_{M' \in \overline{\mathcal{P}^{|E_2|}} \text{ with } \mathscr{B}_{D_2}(M') = \mathscr{B}_{D_2}(M_2)} \mathbb{P}_{D_2, \psi}(M') \times \frac{1}{|[M_2]|}\\
        &= \mathbb{P}_{D_2, \psi}(M_2)
    \end{align*}
    This first step is by definition of the simulation; to get $M_2$, we first have to get an $M_1$ that flips the same costabilisers and then sample from all measurement in $D_2$ that live in the same branch. 
    The second step was shown above. 
    The final step follows from all values in the branch of $M_2$ being equally likely \autoref{prop:equally-likely}.

    The fact that there exists a $P_{M_1, M_2}$ such that $P_{M_1, M_2} D_1^{M_1} = D_2^{M_2}$ follows trivially by the same reasoning as \autoref{prop:pauli-correction}.
\end{proof}

Therefore, we have shown that running $D_1$ is essentially the same as running $D_2$; we get the same distribution over the measurement outcomes and, up to a Pauli correction, the same resulting state. 
In other words, it does not matter which one we run, up to some classical sampling and Pauli corrections, the outcome will be the same.

\subsubsection{ZX Diagrams and Quantum Circuits}
One key difference between measurements as defined above and measurements in quantum circuits is that not all edge flips are valid on all edges. 
In a quantum circuit, we can only get effects that correspond to specific edge flips on edges near the measurements. 

However, we can proof the following: 
\begin{proposition}
    For a quantum circuit, if we only allow the subset of edge flips specified above, we can still reach the same branches as if we allowed all edge flips on all edges.
\end{proposition}
\begin{proof}
    \todo[inline]{check language and clean up}
    We prove by induction on the number of gates that every ZX diagram derived from a circuit possesses a generating set of costabilizing Pauli webs $\mathcal{S}_c$ and a set of measurement flips ${M_{S_i}}$ satisfying the commutation relation $[M_{S_i}, S_j] = \delta_{ij}$.
    For an identity circuit with zero gates, the set of costabilisers is empty, and the claim holds trivially.
    Assume the claim holds for a circuit $C^k$ with $k$ gates with costabiliser generators $\mathcal{S}_c^k$ and respective measurements ${M_{S_i}^k}$.
    If the $(k+1)$-th gate is unitary, the costabilizing group is unchanged, and the inductive hypothesis holds.
    If the $(k+1)$-th gate is a measurement that measures an existing stabiliser of $C^k$, no new costabilisers are introduced, and the hypothesis remains satisfied.
    If the $(k+1)$-th gate measures a logical operator of $C^k$, a new costabiliser $S_n$ is added to the generating set.
    To ensure $S_n$ commutes with all previous measurement flips ${M_{S_i}^k}$, we update $S_n$ by multiplying it by any $S_i \in \mathcal{S}_c^k$ with which it anticommutes.
    We define the new measurement flip $M_n$ as the Pauli operator corresponding to the outcome flip of the $(k+1)$-th gate.
    By construction, $M_n$ anticommutes with $S_n$ but commutes with all $S_i \in \mathcal{S}_c^k$, as the latter are supported only on the previous $k$ gates.
    The expanded set $\mathcal{S}_c^k \cup {S_n}$ and the corresponding measurements ${M_{S_i}^k} \cup {M_n}$ therefore satisfy the required conditions for \autoref{prop:measurement-completeness}.
    This completes the inductive step and the proof.
\end{proof}

As we can reach all branches with the restricted set of measurement outcomes, all proofs about mutual simulation work exactly the same. 

\subsubsection{Mutual Simulation of Quantum Circuits}
Having set-up the theory for mutual simulation, we can now show how to use equivalent circuits to simulate each other. 
In particular, we are interested in the scenario, where we have an idealised specification, we would like to run and, instead, we have a fault-equivalent circuit. 
Said circuit may have substantially more measurements than the specification, meaning, we have to take the measurement circuits of the implementation and figure out what we would have gotten, if we had run the idealised specification. 

Following the proof of \autoref{thm:mutual-simulation}, we need to calculate the branch that our implementation lives in and sample from all measurement outcome that are in the same branch. 
Using the ZX calculus, we can systematise and simplify this process by using parameterised spiders. 
We can add boolean parameters to our diagram along with constraints on these parameters such that for all valid values of the parameters, the two diagrams are the same. 
If we then rewrite our implementation back to the specification, we can track how the measurement outcomes are related. 
Furthermore, we will get the Pauli corrections up to which measurement outcomes in the same branch are equal.

A simple example of two equivalent diagrams is a teleportation circuit which is the same as the identity:
\[\tikzfig{appendix/teleportation-equivalence}\]

Parameterising the edge flip corresponding to the measurement on the teleportation, we get: 
\[\tikzfig{appendix/teleportation-rewrite}\]

From this derivation, we can now read-off how to simulate the identity using the teleportation. 
We observe that both diagrams implement the identity and therefore have no costabilisers. 
As such, there is only one branch. 
Thus, to simulate the identity from the teleportation, we get one measurement outcome which will place us in the one existing branch that does not flip any costabilising Pauli webs.
As the identity has no measurements, there is only one valid measurement outcome in that branch --- namely the trivial one. 
Uniformly sampling from a set of size one will give us that trivial measurement outcome. 
To ensure that the two diagrams implement the same linear map, we finally have to correct the measurement outcome on the teleportation giving us a conditional Pauli $Z$.
Therefore, if we perform the teleportation and do the according correction, it is as if we had done the identity. 

As we know that simulation is bidirectional, we could also use the identity to simulate the teleportation. 
On the other hand, we can also go the other way around; we can perform the identity and up to a Pauli correction, it will be as if we did the teleportation.
When we do the identity, we get no measurement outcomes, placing us in the trivial branch. 
Now, for the teleportation, there will be two measurement outcomes that live in that branch; $0$ and $1$. 
We uniformly sample from both values and do the according correction. 
If we had done the teleporation, we would have similarly gotten $0$ or $1$ with equal probability and, after the Pauli correction, would have also had the same resulting quantum state. 
Therefore, it will be indistinguishable which of the two circuits happened. 

A slightly more interesting example is Shor-style syndrome extraction, which implements the idealised measurement diagram. 
We have: 
\[\tikzfig{appendix/simulation-examples/shor-to-spec}\]
We can see that both diagrams have one costabiliser. 
Whether we live in the $+1$ or $-1$ eigenspace of that costabiliser is determined by the parity of $k_1, k_2, k_3$ and $k_4$ on $D_{shor}$.
On $D_{spec}$ it is decided by the value of $k$.
There are no Pauli corrections needed. 

Thus, when running $D_{shor}$, to get the value that we would have gotten on $D_{spec}$, we can simply take the parity of the four outcomes. 
On the other hand, if we ran $D_{spec}$, we could get one outcome that we would have gotten on $D_{shor}$ by sampling from all measurement outcomes such that $k_1 \oplus k_2 \oplus k_3 \oplus k_4 = k$. 

As a slightly more complicated example, we can consider the optimised implementation of Shor's syndrome extraction. 
As it includes the cat-like linear map, it has more measurements and does need Pauli corrections: 
\[\tikzfig{appendix/simulation-examples/optimised-shor-is-spec}\]
Here, whether we live in the $+1$ or $-1$ eigenspace of the costabiliser of the measurement is determined by the parity of $k_1$ and $k_2$. 
The measurement outcomes $k_3$ and $k_4$ have no effect on the branch the circuit is in. 
However, they live in a shared detecting region, and, therefore, have to have a parity of $0$, as indicated by the free-floating spider.
Thus, their measurement outcome is completely random, as long as $k_3 = k_4$.
While they have no effect on the branch the circuit lives in, they do have an effect on the linear map the circuit implements. 
Therefore, we have to perform a Pauli correction of $Z^{k_3} \otimes I \otimes Z^{k_4} \otimes I$.

\subsubsection{On the Limits of Simulation}
It is essential to remark that simulation is for the fault-free execution of diagrams. 
If faults occur, mutual simulation becomes more complicated. 
In particular, noisy simulation has to be separated into two steps; (1) decoding and (2) noise-free simulation. 

We can view decoding as, given a syndrome, identifying the most likely edge flip with that syndrome such that applying the edge flip once again gives us a syndrome-free circuit.
Once we have decoded, we can once more apply the simulation procedure outlined above, which maps valid measurement outcomes to valid measurement outcomes.
For noise-free simulation, we can use the one process and linear classical compute to create the effect of the other process. 
It would be desirable for something similar to be possible for decoding; given an efficient decoder for one process, efficiently decode the other. 
This is, however, not generally possible \parencite{schweikart}. 
Fault-equivalent rewrites can introduce and remove detecting regions, fundamentally changing the decoding problem. 
Therefore, in general, we can not expect any guarantees for the decoding problem of one circuit given the decoding problem for an equivalent one. 

To simulate one circuit in a noisy setting, given another, we have to tackle the decoding problem from scratch. 
There are settings in which it is relatively easy to calculate the updated decoder \parencite{schweikart, ultra-low-overhead}, however, to the best of our knowledge, this is not possible in general.
Thus, to run one circuit instead of the other, in the noisy setting, one has to recompute the decoding problem from scratch, e.g., using Pauli webs \parencite{ruschCompletenessFault2025}, and create a completely new decoder.
Once a given noisy instance is decoded, one can use the simulation above.

\subsection{Fault Equivalence}
\todo[inline]{I have the notes from the previous version of this write-up but they have to be adapted for the branch notation}
The final definition, we have to prove correct is fault equivalence. 
We have shown that we can think about equivalent circuits as mutually simulating each other, meaning that we run one circuit but, with a little bit of post-processing, we get the same information as if we had run the other circuit. 
We will now show that if two circuits are fault-equivalent, then if we run one circuit under noise, for any fault that can occur, there is an equivalent fault that could have occurred on the other circuit to give the same results. 

\begin{definition}[Fault-equivalence]
    \label{def:fault-equivalent-non-determinisitic}
    Let $D_1$ and $D_2$ be equivalent diagrams with respective simulation information $M_{D_1 \to D_2}$, $\{P_{M_1, M_2}\}$ and $M_{D_2 \to D_1}$, $\{P_{M_2, M_1}\}$.
    Then we say that $D_1$ is fault-equivalent to $D_2$, if for every fault $F_1 \in valid_{D_1}$, there exists a fault $F_2 \in valid_{D_2}$ such that $wt(F_2) \leq wt(F_1)$ and for all input states $\psi$, we have: 
    \begin{itemize}
        \item running $D_1^{F_1}$ on $\psi$ with measurement outcome $M_1$ and then uniformly sampling from $M_{D_1 \to D_2}(M_1)$ is like sampling from $\mathbb{P}_{D_2^{F_2}, \psi}$
        \item for all $M_1 \in valid_{D_1}$ and $M_2 \in M_{D_1 \to D_2}(M_1)$, we have: 
    \end{itemize}
    \[\tikzfig{appendix/faulty-simulation-statement}\]
    and the same holds for all $F_2 \in valid_{D_2}$.
\end{definition}

\begin{proposition}
    Let $D_1$ and $D_2$ be ZX diagrams with respective complete measurement outcomes $\mathcal M_1, \mathcal M_2$ and noise models $\mathcal{F}_1, \mathcal{F}_2$.
    Then, if $D_1$ is fault-equivalent to $D_2$ according to \autoref{def:fault-equivalence}, $D_1$ is also fault equivalent to $D_2$ according to \autoref{def:fault-equivalent-non-determinisitic}.
\end{proposition}
\begin{proof}
    ASs$D_1$ and $D_2$ are fault equivalent according to \autoref{def:fault-equivalence}, we know that $D_1^I = D_2^I$, as the trivial fault is the only fault of weight $0$ on either circuit. 
    Thus, for $F_1 = I$, there must exist a fault of weight $0$ on $D_2$ such that $D_1^I = D_2^F$.

    But then, by \autoref{thm:equivalence}, we know that there exits $M_{D_1 \to D_2}$, $\{P_{M_1, M_2}\}$ and $M_{D_2 \to D_1}$, $\{P_{M_2, M_1}\}$ such that $D_1$ and $D_2$ can respectively simulate each other. 

    Let $F_1 \in valid_{D_1}$. 
    This means that $F_1$ must be undetectable.
    Thus, according to $D_1$ and $D_2$ being fault equivalent, there must exist a fault $F_2$ on $D_2$ such that $D_1^{F_1} = D_2^{F_2}$ and $wt(F_2) \leq wt(F_1)$. 
    As $D_1^{F_1} = D_2^{F_2}$, this means that $F_2$ must also be undetectable and thus $F_2 \in valid_{D_2}$. 

    Finally, we will show that running $D_1^{F_1}$ with corrections $M_{D_1 \to D_2}$ and $\{P_{M_1, M_2}\}$ is like running $D_2^{F_2}$. 
    By \textcite{ruschCompletenessFault2025}, we know that for all undetectable $F_1$, there exist $P_I^{F_1}$ and $P_O^{F_1}$ such that: 
    \[\tikzfig{appendix/pushing-out}\]
    Furthermore, as $D_1^{F_1} = D_2^{F_2}$, $P_I^{F_1}$ and $P_O^{F_1}$ must further satisfy the same for $D_2$:
    \[\tikzfig{appendix/pushing-out-D2}\]

    But then, for all normalised input states $\psi$, we can observe that: 
    \[\tikzfig{appendix/noisy-sampling-distribution}\]
    Analogously, it follows that $\mathbb{P}_{D_2^{F_2}, \psi}(M_2)$ = $\mathbb{P}_{D_2,P_I^{F_1} \psi}(M_2)$.
    But as $P_I^{F_1} \psi$ is still a normalised input state, by $D_1$ being able to simulate $D_2$, we now know that sampling $M_1$ from $\mathbb{P}_{D_1^{F_1}, \psi}$ and then uniformly sampling from $M_{D_1 \to D_2}(M_1)$ is like sampling from $\mathbb{P}_{D_2^{F_2}, \psi}$.

    Finally, we can show that for all $M_1 \in valid_{D_1}$ and $M_2 \in M_{D_1 \to D_2}(M_1)$, we have: 
    \[\tikzfig{appendix/faulty-simulation-statement}\]
    We have: 
    \[\tikzfig{appendix/faulty-simulation-map-proof}\]
    The second step follows from Paulis either commuting or anticommuting.
    The third step follows form $D_1$ simulating $D_2$ and the final step is the reverse of the first step, however, now on $D_2$.
\end{proof}
